# Supplementary material for: Targeted Supervised Contrastive Learning for Long-Tailed Recognition
Source: arXiv:2111.13998 source file (2022-05-02)
Supplement: Supplementary file 1 [file implementations.tex]

\section*{Appendix A: Implementation Details}
In this section, we provide the implementation details of the models used in our experiments. On each dataset, we fix the batch size and training epochs for different baselines based on contrastive loss for a fair comparison. Code will also be released upon acceptance of the paper.

\textbf{CIFAR-10-LT and CIFAR-100-LT}: We build \name~on top of SimCLR-based supervised contrastive learning on CIFAR-10-LT and CIFAR-100-LT \cite{khosla2020supervised}, with a ResNet-32 structure \cite{yang2020rethinking}. All experiments on CIFAR are performed on 4 NVIDIA Titan X Pascal GPUs. For the first stage, the encoder is trained for 1000 epochs with batch size 1024. The learning rate is set to 0.5 initially and decreased using cosine annealing strategy. For the second stage, the linear classifier is trained for 200 epochs with LDAM loss and class re-weighting with batch size 128. The learning rate is set to 0.1 initially and multiplied by 0.1 at epoch 140, 180 and 190.

\textbf{ImageNet-LT and iNaturalist}: We build \name~on top of MoCo-based supervised contrastive learning on ImageNet-LT and iNaturalist \cite{kang2020exploring}, with a ResNet-50 structure \cite{kang2020exploring, yang2021delving}. All experiments on them are performed on 8 NVIDIA Titan X Pascal GPUs. For the first stage, the encoder is trained for 400 epochs with batch size 256. The learning rate is set to 0.1 initially and decreased using cosine annealing strategy. For the second stage, the linear classifier is trained for 40 epochs with with CE loss and class-balanced sampling with batch size 2048. The learning rate is set to 10 on ImageNet-LT and 30 on iNaturalist initially and multiplied by 0.1 at epoch 20 and 30.
