# Supplementary material for: Targeted Supervised Contrastive Learning for Long-Tailed Recognition
Source: arXiv:2111.13998 source file (2022-05-02)
Supplement: Supplementary file 2 [file results.tex]

\section*{Appendix B: Additional Results}
In this section, we provide additional results to better understand \name.

\begin{table}[h]
    \centering
\resizebox{.35\textwidth}{!}{
\begin{tabular}{l|c|c}
\toprule
         & CIFAR-10-LT & CIFAR-100-LT \\
\midrule
LDAM-DRW\cite{cao2019learning} & 77.1 & 42.3 \\
KCL\cite{kang2020exploring} & 77.6  & 42.8  \\
\name & \textbf{79.7}  & \textbf{43.8}  \\
\bottomrule
\end{tabular}}
    \caption{Comparison among LDAM-DRW\cite{cao2019learning}, KCL\cite{kang2020exploring} and \name\ on CIFAR-10-LT and CIFAR-100-LT for 1000 training epochs.}
    \label{tab:longer-epoch}
\vspace{-15pt}
\end{table}

\begin{table}[h]
    \centering
    \resizebox{.2\textwidth}{!}{
    \begin{tabular}{l|c|c}
\toprule
Epochs         & 200 & 400 \\
\midrule
KCL\cite{kang2020exploring} & 51.5  & 51.6  \\
\name & \textbf{52.3}  & \textbf{52.4}  \\
\bottomrule
\end{tabular}}
    \caption{Comparison between KCL\cite{kang2020exploring} and \name\ on ImageNet-LT for 200 and 400 training epochs.}
    \label{tab:kcl-epoch}
\vspace{-15pt}
\end{table}

\textbf{Number of traning epochs}: It is standard in the literature to have a longer training time for contrastive learning than non-contrastive learning because it converges more slowly \cite{chen2020simple, he2020momentum, kang2020exploring, khosla2020supervised}. In Sec. 4, we followed the original paper on supervised contrastive learning\cite{khosla2020supervised} to use 1000 epochs for CIFAR-LT, for both KCL and \name. Here, we also compare with the results of training LDAM-DRW\cite{cao2019learning} for 1000 epochs on CIFAR-10-LT and CIFAT-100-LT ($\rho=100$). As shown in Table~\ref{tab:longer-epoch}, training for longer epochs does not change the results for LDAM-DRW\cite{cao2019learning}. 

In Sec. 4, we used 200 epochs for KCL because the original KCL paper uses 200\cite{kang2020exploring}. We used 400 epochs for \name\ because half of \name's epochs are for warm-up. Since \name\ uses KCL for the warm-up, we started \name\ after KCL has converged, i.e., after 200 epochs, and ran it for another 200 epochs. Here we also report the accuracy of \name\ and KCL on ImageNet-LT for 200 and 400 epochs. As shown in Table~\ref{tab:kcl-epoch}, in both cases, \name\ outperforms KCL.

\begin{table}[h]
% \tablestyle{12.0pt}{1.1}
\caption{Performances of \name~, KCL and cross entropy loss on full CIFAR-10, CIFAR-100 and ImageNet.}
\vspace{-5mm}
\label{tab:full}
\begin{center}
\resizebox{.41\textwidth}{!}{
\begin{tabular}{c|cccc}
\toprule
Methods  & CIFAR-10 & CIFAR-100 & ImageNet \\ 
\midrule
CE           & 92.8  & 71.1 &  76.6   \\
KCL$\dagger$ & 93.0  & 70.5 &  77.0  \\
\name        & 92.9  & 70.8 &  77.1  \\
\bottomrule
\end{tabular}
}
\end{center}
\vspace{-15pt}
\end{table}

\textbf{Performance of \name~on balanced datasets}: similar to KCL, \name~can also be applied to balanced datasets. In Table \ref{tab:full}, we compare the performance of \name~vs. KCL and cross entropy loss on CIFAR-10, CIFAR-100 and ImageNet. As shown in the table, \name~achieves similar performance as KCL and cross-entropy loss on balanced datasets, and the improvements are far less than its improvements on imbalanced datasets. This further shows that \name's improvements on imbalanced datasets comes from its ability to balance the feature space when the data distribution is imbalanced.

\begin{table}[h]
\centering
\caption{\name~ with different $\lambda$ on CIFAR-10-LT with imbalance ratio 100.}
\vspace{-5pt}
\label{tab:ablation-lambda}
\resizebox{0.48\textwidth}{!}{
\begin{tabular}{c|c|c|c|c|c|c|c|c|c|c}
\toprule[1.5pt]
$\lambda$ & 0.01    & 0.05    & 0.1   & 0.2   & 0.3   & 0.5    & 1   & 2 & 5   & 10 \\
\midrule
\textsc{Acc (\%)}                  & 78.4 & 79.2 & 79.6 & \textbf{79.7} & 79.4 & 79.5 & 78.8 & 78.5 & 78.2 &  78.0  \\\midrule
\bottomrule[1.5pt]
\end{tabular}
}
\end{table}

\textbf{Performance of \name~with different $\lambda$}: In \name, the targeted supervised contrastive loss is a weighted sum of two components, the first is a standard supervised contrastive loss as used in KCL \cite{kang2020exploring}, whereas the second is a contrastive loss between the target and the samples in the batch:
% \begin{align*}
%     \mathcal{L}_{TSC} = -\frac{1}{N} \sum_{i=1}^N \Big(\frac{1}{k+1}\sum_{v_j^+ \in \Tilde{V^+_{i, k}}} & \log \frac{e^{v_i^T\cdot v_j^+/\tau}}{ \sum\limits_{v_j\in \Tilde{V_i} \cup U} e^{v_i^T\cdot v_j/\tau}}\\
%     + \lambda & \log \frac{e^{v_i^T\cdot t^*_{\sigma^*_{y_i}}/\tau}}{ \sum\limits_{v_j\in \Tilde{V_i} \cup U} e^{v_i^T\cdot v_j/\tau}}\Big).
% \end{align*}
\begin{align*}
    \mathcal{L}_{TSC} = -\frac{1}{N} \sum_{i=1}^N \Big(&\frac{1}{k+1}\sum_{v_j^+ \in \Tilde{V^+_{i, k}}}  \log \frac{e^{v_i^T\cdot v_j^+/\tau}}{ \sum\limits_{v_j\in \Tilde{V_i} \cup U} e^{v_i^T\cdot v_j/\tau}}\\
    &+ \lambda  \log \frac{e^{v_i^T\cdot c^*_i/\tau}}{ \sum\limits_{v_j\in \Tilde{V_i} \cup U} e^{v_i^T\cdot v_j/\tau}}\Big)
\end{align*}

In the experiments of main paper, $\lambda$ is set to 0.2. In this section, we investigate how different $\lambda$ affects the performance of \name. Table \ref{tab:ablation-lambda} compares the performance of \name~ with different $\lambda$ on CIFAR-10-LT with imbalance ratio 100. As we can see from the results, \name\ is robust to a wide range of values for $\lambda$. In particular, values between $0.1$ and $0.5$ all yield very good performance, with the best being $0.2$. With smaller values, the performance drops slowly this is because a too small $\lambda$ may not be enough to pull the samples to the targets. We also notice that with large $\lambda$, there is too much emphasis on pulling each class to the nearest target and less emphasis on keeping the classes that are semantically clause near each other.   Therefore, we fix $\lambda=0.2$ for all experiments.

\begin{table}[h]
% \tablestyle{12.0pt}{1.1}
\caption{\name~with and without warm-up on ImageNet-LT.}
\vspace{-5mm}
\label{tab:warmup}
\begin{center}
\resizebox{.45\textwidth}{!}{
\begin{tabular}{c|ccccc}
\toprule
Methods  & Many & Medium & Few & All & \textbf{R}$^\downarrow$\\ 
\midrule 
w/o warmup & 62.1 & 48.9 & 29.3 & 51.3 & 7.65 \\
w/ warmup & \textbf{63.5} & \textbf{49.7} & \textbf{30.4} & \textbf{52.4} & \textbf{7.14} \\
\bottomrule
\end{tabular}
}
\end{center}
\vspace{-20pt}
\end{table}

\textbf{Warm-up Training.} As mentioned in Sec. 4.1, we first warm up the network by not assigning targets and simply training the network with the KCL loss. As shown in Table \ref{tab:warmup}, a network trained with a warm-up phase achieves much better accuracy and reasonability than without warm-up on ImageNet-LT. This is likely because in the early stage of training, the feature space is quite random. As a result, the class target assignment at such early stages is nearly random assignment and thus could prevent the feature space from learning good semantics.

\begin{figure}[h]
\begin{center}
%\includegraphics[width=\linewidth]{pos-neg}
%\vspace{-15pt}
\includegraphics[width=0.45\textwidth]{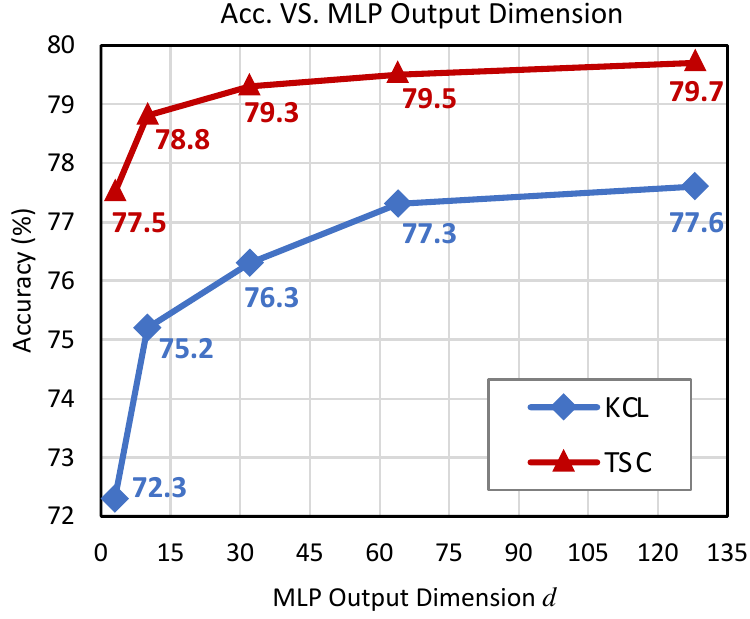}
\end{center}
\vspace{-10pt}
\caption{Comparison of KCL and \name~on different output feature dimensions $d$ on CIFAR-10-LT with imbalance ratio 100.}
\label{fig:dimension}
\vspace{-10pt}
\end{figure}

\textbf{Output Dimensions.} One important hyper-parameter of contrastive learning is the output dimension of the MLP head. In all of our experiments, we set the default output dimension to be 128. In Fig. \ref{fig:dimension}, we compare the performance of \name~and KCL with different MLP output dimensions on CIFAR-10-LT with imbalance ratio 100. As shown in the figure, the performance of \name~is quite robust to small output dimensions (77.5\% at $d=3$ and 79.6\% at $d=128$), while KCL experiences noticeable performance drop when the output dimension is small (only 72.3\% at $d=3$ and 77.6\% at $d=128$). This is possibly because when the output dimension is small, it is harder for KCL to achieve good uniformity, while \name~always achieves good uniformity because of the pre-computed targets.
